# Supplementary material for: Quantitative analysis of single particle trajectories: mean maximal excursion method
Source: arXiv:1001.4412 source file (2010-01-25)
Supplement: Supplementary file 1 [file suppl.pdf]

# Supplementary material, Tejedor et al

In this Supplementary material we define the simulations procedure used to obtain the time series analyzed in the main text. We also collect the supporting calculations for the quantities presented in the main text. Moreover we provide a background for the experimental data analysed in the main text.

## I. SIMULATIONS PROCEDURE

We generated time series of two-dimensional random walks by simulation of each of the three subdiffusion models. The dimensionality mimics the fact that typically 2D trajectories are recorded in experiments. The anomalous diffusion exponent in each case was chosen as $\alpha = 0.7$, a value observed in a number of biological contexts [1–6]. For each model we create 1,000 trajectories, each containing 100 steps. In the CTRW case we perform a 2D Monte Carlo random walk with a stable waiting distribution of the form $\psi(t) \sim \frac{\alpha\tau^\alpha}{\Gamma(1-\alpha)t^{1+\alpha}}$ ($\alpha \simeq 0.70$), and Gaussian jump length statistics of width $\langle\delta\mathbf{r}^2\rangle^{1/2} = 1$. To simulate diffusion on a fractal we generate Monte Carlo random walks on a 2D critical link percolation cluster of size $250 \times 250$ ($d_f = 91/48$ and $d_w \approx 2.844$, so that $\alpha = 2/d_w \simeq 0.70$). Finally, in the FBM case we use the Hosking method [7] to generate a 2D-FBM with an exponent $H = 0.35$ ($\alpha = 2H = 0.70$). We point out that FBM and CTRW are simulated in a free environment (no boundaries), while the percolation network is, by definition, in a confined environment. Since we chose small time intervals in the analysis, this will not significantly affect our results.

The purpose of the simulations is to generate subdiffusion time series of specific models. This enables us to prove that the tools developed in this work are indeed capable to distinguish these mechanisms. The data sets are chosen relatively small in order to mimic typical experimental data sets.

## II. GENERAL FORMULAS

We first study the moments for regular Brownian motion. To compute the second and the fourth regular and maximal excursion (MME) moments we use the diffusion equation. In $d$ dimensions and for spherical geometry this reads

$$\frac{\partial P(r,t)}{\partial t} = \frac{K_1}{r^{d-1}}\frac{\partial}{\partial r}\left(r^{d-1}\frac{\partial P(r,t)}{\partial r}\right). \tag{1}$$

$K_1$ is the diffusion coefficient of dimension cm$^2$/sec.

### A. Regular moments

To compute the regular moments, we impose the normalization and initial conditions

$$\int_0^\infty P(r,t)r^{d_f-1}dr = 1 \text{ and } P(r,0) = \frac{\delta_+(r)}{r^{d_f-1}}, \tag{2}$$

where $\delta_+(r)$ is the one-sided $\delta$ function. The boundary conditions are natural, i.e., chosen such that $P(r \to \infty, t) = 0$. After obtaining an expression for the propagator $P(r,t)$ we compute the $n$th moment

$$\langle r^n\rangle = \int_0^\infty r^n P(r,t)r^{d_f-1}dr. \tag{3}$$

Alternatively, this can be obtained by integration of $r^n$ times the diffusion equation.

### B. MME moments

We first calculate the probability that at time $t$ the distance from the origin traveled by the random walker is less than $r_0$: $r_{\max} \le r_0$. To this end we consider an absorbing sphere at the radius $r = r_0$ and obtain the propagator in the domain $0 \le r \le r_0$ using the following boundary and initial conditions:

$$P(r_0,t) = 0 \text{ and } P(r,0) = \frac{\delta_+(r)}{r^{d_f-1}}. \tag{4}$$

The role of the absorbing sphere is to remove the cumulative probability that the random walker actually crossed the distance $r_0$ before $t$. The sought MME probability then becomes

$$\Pr\left(r_{\max} \le r_0, t\right) = \int_0^{r_0} P(r,t)r^{d_f-1}dr. \tag{5}$$

The $n$th MME moment is obtained by integration of $r_{\max}^n$ times the derivative of the cumulative distribution, i.e., the density,

$$\begin{aligned}\langle r_{\max}^n\rangle &= \int_0^\infty r_0^n \frac{\partial\left(\Pr\left(r_{\max} \le r_0, t\right)\right)}{\partial r_0}dr_0 \\ &= n\int_0^\infty r_0^{n-1}\left(1 - \Pr\left(r_{\max} \le r_0, t\right)\right)dr_0. \end{aligned} \tag{6}$$

## III. ONE DIMENSION

The diffusion equation is simply

$$\frac{\partial P(r,t)}{\partial t} = K_1\frac{\partial^2 P(r,t)}{\partial r^2}. \tag{7}$$

After normalization the solution is the well-known Gaussian propagator

$$P(r,t)=\frac{1}{\sqrt{K_1\pi t}}\exp\left(-\frac{r^2}{4K_1t}\right). \quad (8)$$

We then obtain for the second and the fourth moment

$$\langle r^2\rangle = 2K_1t \text{ and } \langle r^4\rangle = 12(K_1t)^2. \quad (9)$$

For an absorbing sphere placed at $r=r_0$ the MME propagator becomes

$$P(r,t)=\frac{2}{r_0}\sum_{n=0}^{\infty}\cos\left(\frac{(2n+1)\pi r}{2r_0}\right)\times\exp\left(-\frac{K_1(2n+1)^2\pi^2t}{4r_0^2}\right). \quad (10)$$

Integrating from 0 to $r_0$ we find the cumulative distribution function

$$\Pr(r_{\max}\le r_0,t) = \frac{4}{\pi}\sum_{n=0}^{\infty}\frac{(-1)^n}{2n+1}\exp\left(-\frac{K_1(2n+1)^2\pi^2t}{4r_0^2}\right). \quad (11)$$

This expression simplifies in the Laplace domain,

$$\Pr(r_{\max}\le r_0,s)=\frac{4}{\pi}\sum_{n=0}^{\infty}\frac{(-1)^n}{2n+1}\frac{1}{s+\frac{K_1(2n+1)^2\pi^2}{4r_0^2}}. \quad (12)$$

We simplify this expression, recalling that

$$\operatorname{sech}(z)=\pi\sum_{n=0}^{\infty}\frac{(-1)^n(2n+1)}{\pi^2(n+1/2)^2+z^2}. \quad (13)$$

The cumulative distribution can therefore be rewritten in the form

$$\Pr(r_{\max}\le r_0,s)=\frac{1}{s}\left[1-\operatorname{sech}\left(r_0\sqrt{\frac{s}{K_1}}\right)\right]. \quad (14)$$

From this expression the Laplace transforms of the second and fourth MME moments become

$$\begin{aligned}
\langle r^2_{\max}(s)\rangle &= \frac{2}{s}\int_0^\infty r_0\operatorname{sech}\left(r_0\sqrt{\frac{s}{K_1}}\right)dr_0 && (15)\\
&= \frac{2K_1}{s^2}\int_0^\infty u\operatorname{sech}(u)du=\frac{4K_1C}{s^2} && (16)\\
\langle r^4_{\max}(s)\rangle &= \frac{4}{s}\int_0^\infty r_0^3\operatorname{sech}\left(r_0\sqrt{\frac{s}{K_1}}\right)dr_0 && (17)\\
&= \frac{4K_1^2}{s^3}\int_0^\infty u^3\operatorname{sech}(u)du && (18)\\
&= \frac{4K_1^2}{s^3}\left(6i(\mathrm{Li}_4(-i)-\mathrm{Li}_4(i))\right). && (19)
\end{aligned}$$

Here $C\approx 0.916$ is Catalan's constant, and $\mathrm{Li}_4$ the polylogarithm. Inverse Laplace transform leads to the following results:

$$\begin{aligned}
\langle r^2_{\max}(t)\rangle &= 4K_1Ct\approx 3.66K_1t && (20)\\
\langle r^4_{\max}(t)\rangle &= \left(12i(\mathrm{Li}_4(-i)-\mathrm{Li}_4(i))\right)(K_1t)^2 && (21)\\
&\approx 23.73(K_1t)^2 && (22)
\end{aligned}$$

| | $\sigma^2=\langle X^4\rangle-\langle X^2\rangle^2$ | $\gamma=\sqrt{\frac{\langle X^4\rangle-\langle X^2\rangle^2}{\langle X^2\rangle^2}}$ |
|---|---|---|
| RM | $8(K_1t)^2$ | 1.41 |
| MME | $10,31(K_1t)^2$ | 0.876 |

TABLE I: Regular and MME moment statistics in 1D.

We compare the variance and the dispersion of regular and MME moments in table I.

## IV. TWO DIMENSIONS

We write the diffusion equation in Cartesian coordinates,

$$\frac{\partial P(x,y,t)}{\partial t}=K_1\left(\frac{\partial^2P(x,y,t)}{\partial x^2}+\frac{\partial^2P(x,y,t)}{\partial y^2}\right). \quad (23)$$

After normalization the solution is

$$P(r,t)=\frac{1}{2K_1t}\exp\left(-\frac{r^2}{4K_1t}\right). \quad (24)$$

The second and fourth moments follow,

$$\langle r^2\rangle=4K_1t \text{ and } \langle r^4\rangle=32(K_1t)^2. \quad (25)$$

To place an absorbing circle at $r=r_0$ we need to pass to spherical coordinates,

$$\frac{\partial P(r,t)}{\partial t}=\frac{K_1}{r}\left(r\frac{\partial^2P(r,t)}{\partial r^2}+\frac{\partial P(r,t)}{\partial r}\right). \quad (26)$$

Rescaling of time by $K_1$ leads to the solution

$$P(r,t)=\sum_{n=0}^{\infty}A_nJ_0(K_nr)\exp\left(-K_1K_n^2t\right), \quad (27)$$

where $A_n$ and $K_n$ are free parameters. Here we chose the Bessel function $J_0$ to ensure strict positivity of the density in $r=0$. The boudary condition $P(r_0,t)=0$ then imposes $K_n=x_{0n}/r_0$ ($x_{0n}$ is the $n$th zero of $J_0$). For the normalization we use the Fourier-Bessel expansion formalism

$$\begin{aligned}
A_n &= \frac{\int_0^{r_0}\frac{\delta(r)}{r}J_0(K_nr)2\pi rdr}{\int_0^{r_0}J_0(K_nr)^2 2\pi rdr}\\
&= \frac{1}{\pi r_0^2J_1(x_{0n})^2}. && (28)
\end{aligned}$$

Integrating $P(r,t)$ from 0 to $r_0$ we find

$$\Pr(r_{\max}\le r_0,t)=\sum_{n=0}^{\infty}\frac{2}{x_{0n}J_1(x_{0n})}\exp\left(-\frac{K_1x_{0n}^2t}{r_0^2}\right). \quad (29)$$

In Laplace space,

$$\Pr(r_{\max}\le r_0,s)=\sum_{n=0}^{\infty}\frac{2}{x_{0n}J_1(x_{0n})}\left(\frac{1}{s+\frac{K_1x_{0n}^2}{r_0^2}}\right). \quad (30)$$

| | $\sigma^2 = \langle X^4\rangle - \langle X^2\rangle^2$ | $\gamma = \sqrt{\frac{\langle X^4\rangle - \langle X^2\rangle^2}{\langle X^2\rangle^2}}$ |
|---|---|---|
| MSD | $16(K_1 t)^2$ | 1 |
| MME | $18.12(K_1 t)^2$ | 0.694 |

TABLE II: Regular and MME moments statistics in 2D.

| | $\sigma^2 = \langle X^4\rangle - \langle X^2\rangle^2$ | $\gamma = \sqrt{\frac{\langle X^4\rangle - \langle X^2\rangle^2}{\langle X^2\rangle^2}}$ |
|---|---|---|
| MSD | $24(K_1 t)^2$ | 0.816 |
| MME | $25.63(K_1 t)^2$ | 0.602 |

TABLE III: Regular and MME moment statistics in 3D.

By a non trivial contour integral (see reference [8] for a complete proof) we finally obtain

$$\Pr(r_{\max} \leq r_0, s) = \frac{1}{s}\left(1 - \frac{1}{I_0\left(r_0\sqrt{\frac{s}{K_1}}\right)}\right). \quad (31)$$

This expression cannot be simplified any further. We compute the second and fourth MME moments numericaly, in Laplace and real space,

$$\langle r_{\max}^2(s)\rangle = \frac{2K_1}{s^2}\int_0^\infty \frac{u}{I_0(u)}du \quad (32)$$

$$\Rightarrow \langle r_{\max}^2(t)\rangle = 2K_1 t\int_0^\infty \frac{u}{I_0(u)}du \quad (33)$$

$$\langle r_{\max}^4(s)\rangle = \frac{4K_1^2}{s^3}\int_0^\infty \frac{u^3}{I_0(u)}du \quad (34)$$

$$\Rightarrow \langle r_{\max}^4(t)\rangle = 2(K_1 t)^2\int_0^\infty \frac{u^3}{I_0(u)}du. \quad (35)$$

Table II summarizes our findings in two dimensions.

## V. THREE DIMENSIONS

The diffusion equation in cartesian coordinates reads

$$\frac{\partial P(x,y,z,t)}{\partial t} = K_1\left(\frac{\partial^2}{\partial x^2} + \frac{\partial^2}{\partial y^2} + \frac{\partial^2}{\partial z^2}\right), P(x,y,z,t). \quad (36)$$

with the normalized solution

$$P(x,y,z,t) = \frac{1}{(4\pi K_1 t)^{3/2}}\exp\left(-\frac{r^2}{4K_1 t}\right), \quad (37)$$

with $r = \sqrt{x^2+y^2+z^2}$. We then obtain for the second and the fourth moments

$$\langle r^2\rangle = 6K_1 t \text{ and } \langle r^4\rangle = 60(K_1 t)^2. \quad (38)$$

To calculate the solution with an absorbing sphere located at $r = r_0$ we turn to spherical coordinates,

$$\frac{\partial P(r,t)}{\partial t} = \frac{K_1}{r^2}\frac{\partial}{\partial r}\left(r^2\frac{\partial P(r,t)}{\partial r^2}\right) = \frac{K_1}{r}\frac{\partial^2 rP(r,t)}{\partial r^2}. \quad (39)$$

The quantity $rP(r,t)$ satisfies the 1D diffusion equation. $rP(r,t)$ can be written in a Fourier expansion, but now the value at $r = 0$ is 0:

$$\frac{\partial P(r,t)}{\partial t} = \sum_{n=1}^{\infty}\frac{2n\pi}{r_0^2}\frac{\sin(n\pi r/r_0)}{4\pi r}\exp\left(-\frac{K_1 n^2\pi^2 t}{r_0^2}\right). \quad (40)$$

Integration from 0 to $r_0$ and Laplace transformation leads to the expression

$$\Pr(r_{\max} \leq r_0, t) = \sum_{n=1}^{\infty} 2(-1)^{n+1}\exp\left(-\frac{K_1 n^2\pi^2 t}{r_0^2}\right) \quad (41)$$

$$\Pr(r_{\max} \leq r_0, s) = 2\sum_{n=1}^{\infty}\frac{(-1)^{n+1}}{s + \frac{K_1 n^2\pi^2}{r_0^2}}. \quad (42)$$

This expression can be simplified by use of a contour integral, obtaining

$$\Pr(r_{\max} \leq r_0, s) = \frac{1}{s}\left(1 - \frac{\sqrt{\frac{s}{D}}r_0}{\sinh\left(\sqrt{\frac{s}{D}}r_0\right)}\right). \quad (43)$$

We deduce the Laplace transforms of the moments, as well as their expression after back transformation to time:

$$\langle r_{\max}^2(s)\rangle = \frac{2K_1}{s^2}\int_0^\infty \frac{u^2}{\sinh(u)}du \quad (44)$$

$$\Rightarrow \langle r_{\max}^2(t)\rangle = 7K_1 t\zeta(3) \quad (45)$$

$$\langle r_{\max}^4(s)\rangle = \frac{4K_1^2}{s^3}\int_0^\infty \frac{u^4}{\sinh(u)}du \quad (46)$$

$$\Rightarrow \langle r_{\max}^4(t)\rangle = 93(K_1 t)^2\zeta(5). \quad (47)$$

Here $\zeta$ represents the Riemann zeta function. The results of the 3D case are summarized in table III.

## VI. ANOMALOUS DIFFUSION

### A. Fractional Brownian motion

The propagator of FBM in free space is [9]

$$P(r,t) = \frac{2}{\Gamma(d/2)\left(4K_\alpha t^\alpha\right)^{d/2}}\exp\left(-\frac{r^2}{4K_\alpha t^\alpha}\right), \quad (48)$$

which is equal to the propagator of Brownian motion after the substitution $t \to t^\alpha$. This expression is in fact the superposition of $d$ FBM processes. From equation (48) we obtain the same results for the regular moments as for Brownian motion, with the analogous substitution for time. The results are collected in table IV. To calculate the MME statistics one would need to know the solution of FBM in the presence of an absorbing boundary, a so far elusive quantity.

We estimated the MME second moment exponent and MME ratio by numerical simulation. We generated 100,000 trajectories of 512 steps length in 2 dimensions,

| | 1 D | 2 D | 3 D |
|---|---|---|---|
| $\langle r^2 \rangle$ | $2K_1 t^\alpha$ | $4K_1 t^\alpha$ | $6K_1 t^\alpha$ |
| $\langle r^4 \rangle$ | $12\,(K_1 t^\alpha)^2$ | $32\,(K_1 t^\alpha)^2$ | $60\,(K_1 t^\alpha)^2$ |

TABLE IV: MSD statistics for FBM.

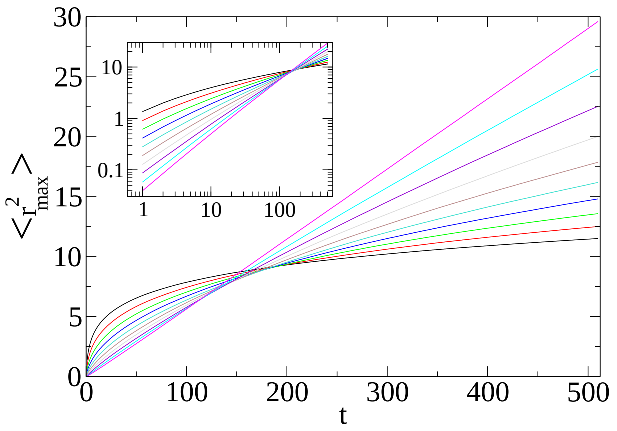


FIG. 1: Second MME moment as a function of time for different FBM in 2 dimensions. Each line correspond to a given value of $H$, between 0.05 and 0.5 (with steps of 0.05), and is averaged over 100,000 trajectories of 512 steps length. The inset is a log-log plot, showing more clearly the power-law behavior, if we except the points for $t < 10$.

using the Hosking method [7]. The $H$ exponent varies from 0.05 ($\alpha = 0.1$) to 0.5 ($\alpha = 1$ corresponding to Brownian motion) in steps of 0.05. We plot in figure 1 the second MME moment as a function of time, observing that it behaves like a power-law for all $H$ values, if we except the initial points where the estimate of $r_{\max}$ is not very accurate. The surprising result is that the exponents are always greater than $\alpha$. We denote by $\alpha'$ the second MME moment exponent, and we list in table V the fitted values of $\alpha$ and $\alpha'$. The $\alpha$ values are always very close to the theoretical one ($2H$), and $H = 0.5$ returns the exponent for Brownian motion ($\alpha = \alpha' = 1$). We see that $\alpha'$ behaves linearly with $\alpha$, a linear regression gives, with a high correlation coefficient:

$$\alpha' \simeq 0.156 \pm 0.005 + (0.849 \pm 0.008)\alpha \qquad (49)$$

Figure 2 shows the MME ratio as a function of time. We here obtain a more classical behavior, with a saturation for long times. This result is not a priori obvious: it means that the fourth MME moment scales as $t^{2\alpha'}$. The saturation value grows with $H$. We note that all curves start from 2 for $t = 1$, which is the MSD ratio in 2D ($r = r_{\max}$ for $t = 1$), and that the upper curves converge toward 1.49, the expected value for a Brownian motion in 2D. We do not have access to the limit $t \to \infty$, so we estimated the ratio using the minimal value, reached at time $t = 512$. Table VI summarizes these results. Since

| $H$ | fitted $\alpha$ ($= 2H$ in theory) | fitted $\alpha'$ |
|---|---|---|
| 0.05 | 0.0991 | 0.2491 |
| 0.10 | 0.1993 | 0.3301 |
| 0.15 | 0.3015 | 0.4114 |
| 0.20 | 0.4003 | 0.4922 |
| 0.25 | 0.5015 | 0.5742 |
| 0.30 | 0.5971 | 0.6561 |
| 0.35 | 0.6979 | 0.7439 |
| 0.40 | 0.7982 | 0.8342 |
| 0.45 | 0.8962 | 0.9231 |
| 0.50 | 0.9975 | 1.0168 |

TABLE V: FBM regular ($\alpha$) and MME ($\alpha'$) second moment exponents in 2D (numerical simulation). Those values are power-law fits of the curves plotted in figure 1: each $H$ value is an average over 100,000 trajectories of 512 steps length.

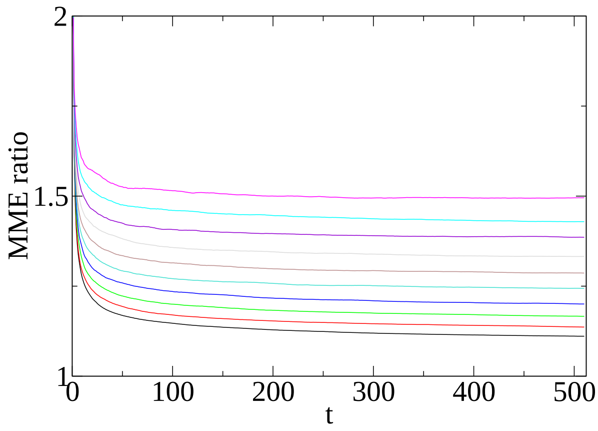


FIG. 2: MME ratio ($\langle r^4_{\max}\rangle / \langle r^2_{\max}\rangle^2$) as a function of time for different FBM in 2 dimensions. Each line corresponds to a given value of $H$, between 0.05 and 0.5, increasing by steps of size 0.05. We average over 100,000 trajectories of 512 steps length.

the precision of the estimation is not very good, it is hard to recognize a particular behavior of this ratio with $H$. We propose a rough approximation using a shifted power-law, to be able to compare to a numerical value for a given $H$:

$$\frac{\langle r^4_{\max}\rangle}{\langle r^2_{\max}\rangle^2} \simeq (1.05 \pm 0.01) H^{1.42 \pm 0.01} + (1.10 \pm 0.01) \quad (50)$$

### B. Continuous time random walk

For an uncoupled CTRW the trajectory is that of a normal Brownian random walk, however, at each step, the random walker becomes immobilized for a random

| $H$ | 0.05 | 0.10 | 0.15 | 0.20 | 0.25 | 0.30 | 0.35 | 0.40 | 0.45 | 0.50 |
|---|---|---|---|---|---|---|---|---|---|---|
| MME ratio | 1.11 | 1.14 | 1.17 | 1.20 | 1.24 | 1.29 | 1.33 | 1.39 | 1.43 | 1.49 |

TABLE VI: FBM MME ratio in 2D (numerical simulation). The values are the minimum reached at time $t = 512$ in figure 2: each $H$ value is an average over 100,000 trajectories of 512 steps length.

waiting time $\tau$. If this waiting time is of the scaling form $\psi(\tau) \simeq \tau_0/\tau^{1+\alpha}$ with $0 < \alpha < 1$ the process is governed by the fractional diffusion equation [10]

$$\frac{\partial P(r,t)}{\partial t} = \frac{K_\alpha}{r^{d-1}}\frac{\partial}{\partial r}\left(r^{d-1}\frac{\partial}{\partial r}\left({}_0D_t^{1-\alpha}P(r,t)\right)\right). \quad (51)$$

Here we used the Riemann-Liouville fractional operator [10]

$${}_0D_t^{1-\alpha}P(r,t) = \frac{1}{\Gamma(\alpha)}\frac{\partial}{\partial t}\int_0^t dt' \frac{P(r,t')}{(t-t')^{1-\alpha}}, \quad (52)$$

which introduces a long-range memory into the process. The generalized diffusion constant $K_\alpha = \langle \delta \mathbf{r}^2 \rangle / [2\tau_0^\alpha]$ is of dimension $\mathrm{cm}^2/\mathrm{sec}^\alpha$, where we used the (finite) jump length variance $\langle \delta \mathbf{r}^2 \rangle$. The Laplace transform of the diffusion equation is therefore

$$sP(r,s) - P(r,0^+) = s^{1-\alpha}\frac{K_\alpha}{r^{d-1}}\frac{\partial}{\partial r}\left(r^{d-1}\frac{\partial}{\partial r}P(r,s)\right). \quad (53)$$

### 1. One dimensional case

In 1D the fractional diffusion equation is

$$sP(r,s) - \delta(r) = s^{1-\alpha}K_\alpha \frac{\partial^2 P(r,s)}{\partial r^2}, \quad (54)$$

where we chose the sharp initial condition $P(r,0) = \delta(r)$. The general solution is

$$\begin{aligned} P(r,s) &= A\sinh\left(\sqrt{\frac{s^\alpha}{K_\alpha}}r\right) + B\cosh\left(\sqrt{\frac{s^\alpha}{K_\alpha}}r\right) \\ &\quad -\sqrt{\frac{s^\alpha}{K_\alpha}}\frac{\Theta(r)}{s}\sinh\left(\sqrt{\frac{s^\alpha}{K_\alpha}}r\right), \end{aligned} \quad (55)$$

where $\Theta(r)$ is the Heaviside step function.

For natural boundary conditions and after renormalization ($\int_0^\infty P(r,s)dr = 1/s$) we find the following solution in Laplace space,

$$P(r,s) = \sqrt{\frac{s^\alpha}{K_\alpha}}\frac{1}{s}\exp\left(-\sqrt{\frac{s^\alpha}{K_\alpha}}r\right). \quad (56)$$

The second and the fourth regular moments in Laplace and time domain follow:

$$\langle X^2(s) \rangle = \frac{2K_\alpha}{s^{1+\alpha}} \Rightarrow \langle X^2(t) \rangle = \frac{2K_\alpha}{\Gamma(1+\alpha)}t^\alpha \quad (57)$$

$$\langle X^4(s) \rangle = \frac{24K_\alpha^2}{s^{1+2\alpha}} \Rightarrow \langle X^4(t) \rangle = \frac{24K_\alpha^2}{\Gamma(1+2\alpha)}t^{2\alpha}. \quad (58)$$

For the MME moments we need to take into account the boundary condition $P(r_0,s) = 0$ and $P(-r_0,s) = 0$,

$$\begin{aligned} \left(A - \sqrt{\frac{s^\alpha}{K_\alpha}}\right)\sinh\left(\sqrt{\frac{s^\alpha}{K_\alpha}}r_0\right) + B\cosh\left(\sqrt{\frac{s^\alpha}{K_\alpha}}r_0\right) &= 0 \\ A\sinh\left(-\sqrt{\frac{s^\alpha}{K_\alpha}}r_0\right) + B\cosh\left(-\sqrt{\frac{s^\alpha}{K_\alpha}}r_0\right) &= 0. \end{aligned} \quad (59)$$

We note that the propagator is parity invariant,

$$P(r,s) = \frac{K_\alpha}{s}\sinh\left(\sqrt{\frac{s^\alpha}{K_\alpha}}r\right)(1 - 2\Theta(r)) \quad (60)$$

$$+\frac{K_\alpha}{s}\tanh\left(\sqrt{\frac{s^\alpha}{K_\alpha}}r_0\right)\cosh\left(\sqrt{\frac{s^\alpha}{K_\alpha}}r\right), \quad (61)$$

as it should be. The cumulative distribution function is obtained by integration from $-r_0$ to $r_0$,

$$\Pr\left(r_{\max} \le r_0, s\right) = \frac{1}{s}\left(1 - \mathrm{sech}\left(\sqrt{\frac{s^\alpha}{K_\alpha}}r_0\right)\right). \quad (62)$$

We finally deduce the second and the fourth MME moments

$$\begin{aligned} \langle r_{\max}^2(s) \rangle &= \frac{2K_\alpha}{s^{1+\alpha}}\int_0^\infty u\mathrm{sech}(u)du = \frac{4K_\alpha C}{s^{1+\alpha}} \\ \Rightarrow \langle r_{\max}^2(t) \rangle &= \frac{4K_\alpha C}{\Gamma(1+\alpha)}t^\alpha \\ \langle r_{\max}^4(s) \rangle &= \frac{4K_\alpha^2}{s^{1+2\alpha}}\int_0^\infty u^3\mathrm{sech}(u)du \\ \Rightarrow \langle r_{\max}^4(t) \rangle &= \frac{12iK_\alpha^2}{\Gamma(1+2\alpha)}(\mathrm{Li}_4(-i) - \mathrm{Li}_4(i))t^{2\alpha}. \end{aligned} \quad (63)$$

### 2. General case

The CTRW propagator in Laplace space is very similar to the analogous expression for Brownian motion. In fact, in the Laplace domain we have a simple mapping between the $d$-dimensional CTRW and $d$-dimensional Brownian motion, as can be seen from the Laplace transform of the fractional diffusion equation,

$$\frac{\partial}{\partial r}\left(r^{d-1}\frac{\partial}{\partial r}P(r,s)\right) - \frac{r^{d-1}s^\alpha}{K_\alpha}P(r,s) = -\frac{s^\alpha}{K_\alpha s}\delta(r). \quad (64)$$

This equation is exactly the same as in the Brownian case if we write $K_1 = K_\alpha s^{1-\alpha}$. This property corresponds to a subordination in the time domain [10–12]. Replacing $K_1$ by $K_\alpha s^{1-\alpha}$ in the previous results produces the expressions in table VII.

## C. Summary

According to the moment ratios we can see that the distribution of the MME statistic is more closely centred

| | 1 D | 2 D | 3 D |
|---|---|---|---|
| $\langle r^2 \rangle$ | $2/\Gamma(1+\alpha)K_\alpha t^\alpha$ | $4/\Gamma(1+\alpha)K_\alpha t^\alpha$ | $6/\Gamma(1+\alpha)K_\alpha t^\alpha$ |
| $\langle r^2_{\max} \rangle$ | $3.66/\Gamma(1+\alpha)K_\alpha t^\alpha$ | $6.14/\Gamma(1+\alpha)K_\alpha t^\alpha$ | $8.41/\Gamma(1+\alpha)K_\alpha t^\alpha$ |
| $\langle r^4 \rangle$ | $24/\Gamma(1+2\alpha)\,(K_\alpha t^\alpha)^2$ | $64/\Gamma(1+2\alpha)\,(K_\alpha t^\alpha)^2$ | $120/\Gamma(1+2\alpha)\,(K_\alpha t^\alpha)^2$ |
| $\langle r^4_{\max} \rangle$ | $47.47/\Gamma(1+2\alpha)\,(K_\alpha t^\alpha)^2$ | $111.59/\Gamma(1+2\alpha)\,(K_\alpha t^\alpha)^2$ | $192.87/\Gamma(1+2\alpha)\,(K_\alpha t^\alpha)^2$ |

TABLE VII: MSD & MME statistics for CTRW.

around its mean than the regular probability distribution $P(x,t)$. This means that the statistics at finite times in the case of MME analysis is improved, compared to the MSD analysis. This in fact reduces the significance of potential outliers, in particular, at shorter times. The effect can be seen in the graphs for the glycerine data in the main text, but also for the other cases: in the analysis of the simulations data the MME reproduces the known exponent more truthfully, and also for the lipid granules the data are less noisy in the MME analysis. We do not have a general analytical estimate of the error in the MME case, but believe that the case studies presented in the main text support our claim of higher accuracy.

## VII. EXPERIMENTAL DATA

We here provide details on the experimental data discussed in the main text. They are from free diffusion of quantum dots and granules in living yeast cells.

### A. Free diffusion of Quantum Dots

The first set of data was obtained from fluorescence video tracking of single quantum dots (Qdot 565 streptavidin conjugate, Invitrogen Corporation, USA) freely diffusing in glycerol (G7757, Sigma Aldrich, USA) at room temperature (25°C) [Simmel lab, TUM]. The quantum dot stock solution was diluted in glycerol to a final concentration of 1 nM prior to usage. Samples were imaged using microscopic chamber slides ($\mu$-slide 8, ibidi GmbH, Germany), which were incubated with 10 mg/ml BSA solution (A-7906, Sigma Aldrich, USA) for 2 h to prevent non-specific adsorption of quantum dots to the surface. Fluorescence imaging was carried out on an inverted fluorescence microscope (IX-71, Olympus Corporation, Japan) in wide field configuration with an oil-immersion objective (PlanApo, 100X, NA 1.45 Oil TIRFM, Olympus Corporation, Japan) corresponding to a pixel size of 160 nm. The illumination light (X-Cite Series 120, EXFO Life Sciences, Canada) was filtered using an excitation bandpass filter (HQ 470/40, AHF Analysetechnik, Germany) and passed through a beam splitter (z 488 RDC, AHF Analysetechnik, Germany). Fluorescence light was filtered with an emission filter (HQ 510 LP, AHF Analysetechnik, Germany) and imaged on an EMCCD camera (Andor iXon+ DU897E, Andor Technology, North Ireland) using a frame rate of 31 fps and an exposure time of 0.03029 s. Single quantum dot trajectories were calculated using the ParticleTracker Plugin [13] for ImageJ [14].

The analysis is based on 67 trajectories, the longest of which consists of 210 frames. For these data, we expect to observe normal Brownian motion.

### B. Granules in yeast cells

In the second set of much longer trajectories (5,500 to 19,400 frames) the particle positions were acquired by video tracking of lipid granules in yeast cells [Oddershede lab, NBI]. We used *Schizosaccharomyces pombe* (*S. pombe*, D817) fission yeast cells, expressing a GFP-fused marker of the nuclear and plasma membrane systems [15]. Spherical lipid granules are endogenously present in the cytoplasm of these cells [16]. The granules are refractive enough to be visualized with bright-field microscopy.

The *S. pombe* fission yeast cells appear cylindrical with outer dimensions of approximately 4 $\mu$m by 12 $\mu$m. The cell is surrounded by a rigid cell wall. The granules which were tracked in the present experiment are densely packed lipids of almost spherical shape and of approximately 300 nm diameter. These granules are located uniformly throughout the cytoplasm, except in the nucleus. The granules perform thermal fluctuations, these fluctuations being somewhat hindered by the presence of cytoskeletal elements such as microtubules, actin, and membranous structures. Due to the coupling to their viscoelastic environment one would expect a subdiffusive behavior of the granules. It is, however, possible that a minority of the granules are actively moved, either by molecular motor transport (though, this has not been proved in literature) or by cytoplasmatic streaming.

The cells were cultured on AA-Leu agar plates for 12-14 hours at 33°C and after growth stored at 4°C. Prior to the experiments, the cells were suspended into liquid AA medium. The fluid chamber for the experiments consisted of two glass slides glued together by a layer of double sticky tape as a spacer. The chamber was then filled with the cell suspension. The cells were allowed to relax on the surface for approximately 20 minutes, so that they do not move during data acquisition. The experiments were performed at room temperature (25°C).

Bright-field microscopy imaging was carried out on a Leica DMIRE2 microscope, using an oil immersion objective (Leica PL Apo 100x), and the AVT Pike F100B camera (Allied Vision Technologies) and the SmartView soft-

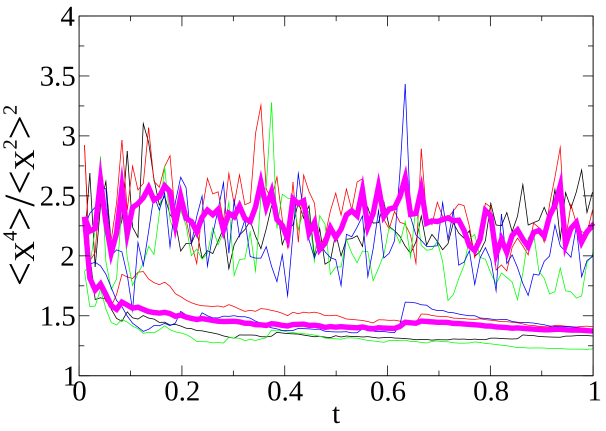


FIG. 3: Lipid granules diffusing in a yeast cell: Ratios $\langle r^4\rangle/\langle r^2\rangle^2$ (upper curves), and $\langle r^4_{\rm max}\rangle/\langle r^2_{\rm max}\rangle^2$ (lower curves) for each trajectory, calculated on subsets of 100 steps pieces. The thick lines represent the ratio for the global set of all the 445 trajectories with 100 steps. The Brownian values are 2 for the upper curves, and 1.49 for the lower ones. Time is in seconds. Note that the scatter in the MME ratios is considerably suppressed in comparison to the regular moments.

ware (Allied Vision Technologies) for recording. Particle tracking was carried out using the PolyParticleTracker Package in Matlab [17]. The error in the determination of the particle position of this method is 20nm.

*Additional graphs for the analysis of the granule motion in yeast cells*

In addition to the analysis shown in the main text we here present two additional graphs further analyzing the granule motion in *S. pombe* yeast cells.

Figure 3 shows the results from the moment ratio analysis. In that course each individual trajectory was split into stretches of 100 steps. For each granule, we then plotted the regular and the MME ratios. They are somewhat noisy, but for each granule the MME ratio is clearly below the Brownian one (1.49): it ranges between 1.20 and 1.40. The regular moment ratio is slightly above the Brownian value (2), between 1.7 and 2.5. We also show in figure 3 the ratio for the whole set of 100 steps pieces (thick lines), which produce approximately the same results as those obtained for individual trajectories. From these ratios, we obtain another clue pointing at an underlying FBM mechanism: the MME moment ratio is, on average, below the value for Brownian motion, and the regular moment ratio close to the Brownian value. These MME ratios are not very precise, but seem to range somewhat above the expected value for FBM with $\alpha = 0.41$, predicted as $1.21 \pm 0.02$ from equation (11) of the main text.

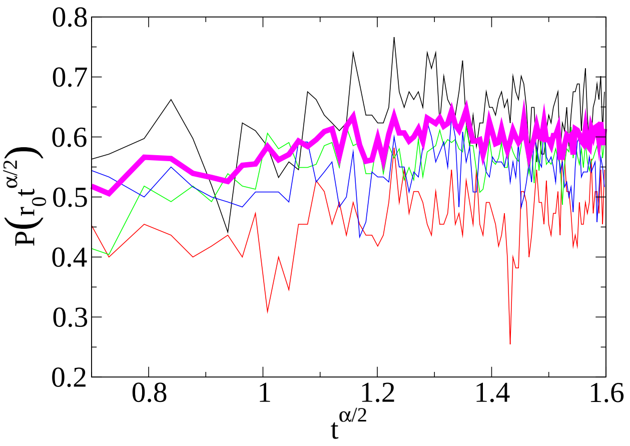


FIG. 4: Lipid granules diffusing in a yeast cell: Analysis of the probability to be in a growing sphere $r_0 t^{\alpha/2}$ as a function of $t$. For each trajectory, this probability is calculated on a subset of 100 steps long trajectories, and the thick line shows the probability for the global set of all the 445 subtrajectories. The theoretical prediction is a scaling $x^{d-d_f}$, which leads to a fitted value $d_f \approx 2$.

Finally figure 4 shows the test with a growing sphere, demonstrating that a constant value is reached. This excludes the possibility that the process corresponds to diffusion on a fractal.


[1] Seisenberger G., M. U. Ried, T. Endreß, H. Büning, M. Hallek, and C. Bräuchle. 2001. Real-time single-molecule imaging of the infection pathway of an adeno-associated virus. Science 294:1929-1932.

[2] Golding I., and E. C. Cox. 2006. Physical nature of bacterial cytoplasm. Phys. Rev. Lett. 96:098102.

[3] Caspi A., R. Granek, and M. Elbaum. 2000. Enhanced diffusion in active intracellular transport. Phys. Rev. Lett. 85:5655-5658.

[4] Caspi A., R. Granek, and M. Elbaum. 2002. Diffusion and directed motion in cellular transport. Phys. Rev. E 66:011916.

[5] Tolić-Nørrelykke I. M., E.-L. Munteanu, G. Thon, L. Oddershede, and K. Berg-Sørensen. 2004. Anomalous diffusion in living yeast cells. Phys. Rev. Lett. 93:078102.

[6] Selhuber-Unkel C., P. Yde, K. Berg-Sorensen, and L. B. Oddershede. 2009. Intracellular diffusion during the cell cycle. Physical Biology 6:025015.

[7] Hosking J.R.M. 1984. Modeling persistence in hydrological time series using fractional differencing. Water Resour. Res. 20:1898-1908.

[8] Drawn M.D. 1995. On the Summation of Fourier and Bessel Series. J. Math. anal. and applic. 193:282-295.

[9] Wang K.G., and C. W. Lung. 1990. Long-time correlation effects and fractal Brownian motion. Phys. Lett. A 151:119-121.

[10] Metzler R., and J. Klafter. 2000. The random walk's guide to anomalous diffusion: a fractional dynamics approach. Phys. Rep. 339:1-77.

[11] Feller W. 1971. An introduction to probability theory and its applications. Wiley, New York. Vol. 2.

[12] Metzler R., E. Barkai, and J. Klafter. 1999. Anomalous diffusion and relaxation close to thermal equilibrium: A fractional Fokker-Planck equation approach. Phys. Rev. Lett. 82:3563-3567.

[13] Sbalzarini I.F., and P. Koumoutsakos. 2005. Feature point tracking and trajectory analysis for video imaging in cell biology. J. Struct. Biol. 151(2):182-195.

[14] Rasband W. S. ImageJ, U. S. National Institutes of Health, Bethesda, Maryland, USA, http://rsb.info.nih.gov/ij/, 1997-2009.

[15] Ding, D. Q., Y. Tomita, A. Yamamoto, Y. Chikashige, T. Haraguchi, and Y. Hiraoka. 2000. Large-scale screening of intracellular protein localization in living fission yeast cells by the use of a GFP-fusion genomic DNA library. Genes to Cells 5:169-190.

[16] Robinow C.F., and J. S. Hyams. 1989. Molecular Biology of the Fission Yeast. Academic Press, New York, p273-330.

[17] Rogers S.S., T. A. Waigh, X. Zhao, and J. R. Lu. 2007. Precise Particle Tracking Against a Complicated Background: Polynomial Fitting with Gaussian Weight. Phys. Biol. 4:220-227.
